# Supplementary material for: Bayesian sampling with BeAtlas, a grid of synthetic Be star spectra I. Recovering the fundamental parameters of \alpha Eri and \beta CMi
Source: arXiv:2309.06168 source file (2023-09-12)
Supplement: Supplementary file 1 [file table_star_disk_models.tex]

\begin{table*}
\centering
\small
\caption{\textsc{BeAtlas} stellar parameters for disk models.}
\label{tab:star_params_disk_models}
\begin{tabular}{l l l l}
\hline\hline
                   &  Parameters                                  & Ranges      & Values/Step                   \\ \hline
ST                 &  Spec. Type                                  & B9 - O8     & B9, B7, B6, B4, B2.5, B1, B0.5, O8    \\
$M_\star$          &  Mass ($\mathrm{M_\odot}$)                   & 3 - 20      & 3, 4, 5, 7, 9, 12, 15, 20     \\
$W$                &  Rotation Rate                               & 0.5 - 0.99  & 0.5, 0.75, 0.85, 0.92, 0.99   \\
$t/t_\mathrm{ms}$  &  Stellar Age                                 & 0 - 1.25       & 0, 0.5, 1, 1.25               \\
\hline
\end{tabular}
\end{table*}
